# Supplementary material for: Non-autoregressive Sequence-to-Sequence Vision-Language Models
Source: arXiv:2403.02249 source file (2025-03-13)
Supplement: Supplementary file 1 [file X_suppl.tex]

\clearpage
\setcounter{page}{1}
\maketitlesupplementary

\section{Model Designs Analysis}
We provide some additional discussions for objective function design and simplified training targets.

\label{sec:q_ctc}
\subsection{Objective Functions Comparison}

\noindent{\bf Cross-Entropy Loss}
Cross-entropy loss can be used as the objective function for non-autoregressive sequence generation, and it classifies each token independently. Token level cross entropy loss introduces strict prediction and GT alignment, and a slight misalignment could intrigue severe penalty to the sequences close to the correct predictions. This strict alignment confuses the model learning, particularly, on target sequences of high diversity, for example, there exist multiple valid captions for an image. Lack of inter-token dependency modeling causes a large solution space ($L^D$, where $L$ is the target sequence length and $D$ is the vocabulary size), and makes the optimization process hard.

\noindent{\bf CTC Loss}
Connectionist Temporal Classification Loss (CTC) was originally proposed in \cite{graves2006connectionist} for Recurrent neural networks (RNNs) to classify speech signal, where sequence alignment is difficult to form between the unsegmented waveform and the sequence of phonemes, constructed by spikes and blanks separating them, and CTC is also adopted in machine translation \cite{libovicky2018end} to handle the length discrepancy between source sentence and the translated sentence. The following URL \cite{hannun2017sequence} points to a website that provides a nice illustration about the motivation and formulation of the CTC loss, applied to sequence modeling in speech recognition. Unlike in the standard cross-entropy loss where {\bf each token} corresponds to one (or multiple) ground truth results and the CE loss is trying to encourage the individual tokens to make the correct prediction by matching with the ground-truth output. So the cross-entropy loss is an element-wise loss for each token, if we know it's ground-truth output. In the Connectionist Temporal Classification Loss (CTC) case, we {\bf no longer} have a known {\bf token-wise ground-truth} output. Instead, we only know {\bf sequence-level ground-truth} output. A solution that is fairly close to the ground-truth in the sequence level might just have one position shifted to the right for each token after a certain location; if a strict CE loss would have been used, its loss can be large. The CTC loss deals with the alignment issue by marginalizing predictions that are only slightly off to the ground-truth by a shift to assign a faith loss. The CTC loss is:
  
\begin{equation}
L_{\rm \text{CTC}}(\theta) = -  \sum_{k}  \sum_{z_i \sim 
\tilde{p}(z|x_k)} \text{log}\frac{f_{y_i}(z_i(x_k))}{\sum_j e^{f_{y_j}(z_i(x_k))}}
\label{eq:ctc}
\end{equation},
where $\theta$ denotes the learnable parameters of the model, $\tilde{p}(z|x_k)$ denotes the collapsed valid sequences, $f_{y_i}(\cdot)$ computes the
logits of $x_i$ on target token class $y_i$, $k$ is the number of all training samples. $z_i(x_k)$ denotes the ``path" from the input tokens to
the output tokens, meaning the value of $z_i$ as a (deterministic)
function of the encoding $x_k$.

When implementing the CTC loss, there are certain techniques that have been adopted. For example, since there can be stretches for the same character output or multiple consecutive same character (or sub-words if the basic output element is subword), a blank token is introduced to differentiate between the two cases. A post-process is done to remove blank tokens to produce the sequence output. Some illustration can be found at  \cite{hannun2017sequence}. 

\begin{table*}[t]
  \centering
  \scalebox{0.85}{
  \begin{tabular}{ | c | m{10cm} | }
    \hline
    Images & Captions \\ \hline
    \begin{minipage}{.3\textwidth}
      \includegraphics[width=\linewidth]{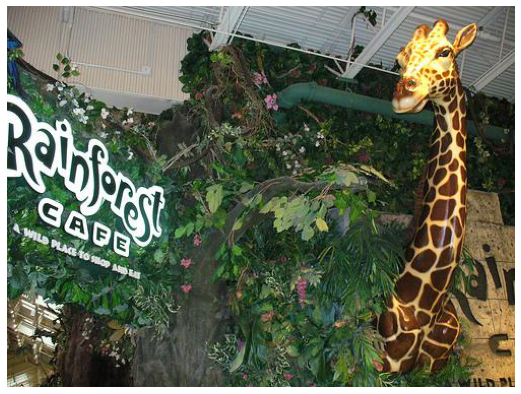}
    \end{minipage}
    &
    %\begin{minipage}[t]{5cm}
      \begin{itemize}
        \item \textbf{Simplified Caption}: A giraffe statue in a room with plants.
        \item \textbf{GT-1}: A fake giraffe standing beside a bunch of trees.
        \item \textbf{GT-2}: A forest like place to go and eat food. 
        \item \textbf{GT-3}: A fake giraffe that is hanging on the side of a wall.
        \item \textbf{GT-4}: A large giraffe standing in the middle of a rainforest cafe.
        \item \textbf{GT-5}: A giraffe bust hanging by a rain forest cafe sign.
      \end{itemize}
    %\end{minipage}
    \\ \hline
  
     \begin{minipage}{.3\textwidth}
      \includegraphics[width=\linewidth]{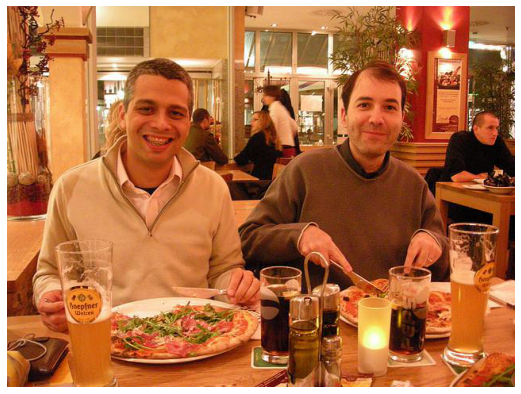}
    \end{minipage}
    &
    %\begin{minipage}[t]{5cm}
      \begin{itemize}
        \item \textbf{Simplified Caption}: Two men sitting at a table eating pizza.
        \item \textbf{GT-1}: Two guys in a bar eating pizza and drinking beer.
        \item \textbf{GT-2}: Two men are sitting side by side as they are eating and smiling, they both are cutting their food with a knife. 
        \item \textbf{GT-3}: Two men sitting at a table eating pizza.
        \item \textbf{GT-4}: Two young men sitting next to each other sharing a meal.
        \item \textbf{GT-5}: Two man sit at a table in a restaurant.
      \end{itemize}
    %\end{minipage}
    \\ \hline 
    
  \end{tabular}
  }
  \caption{Simplified Captions vs GT Captions. We run the autoregressive model on the training dataset to get simplified captions. Each image is annotated by 5 annotators thus we have GT-1 to GT-5 captions. We see that the diversity of original GT output sequences is higher than simplified target sequences.}\label{table:distill_cap}
\end{table*}

\begin{figure}[!ht]
%\vspace{-15mm} 
\begin{center}
\begin{tabular} {c}
\includegraphics[width=0.35\textwidth]{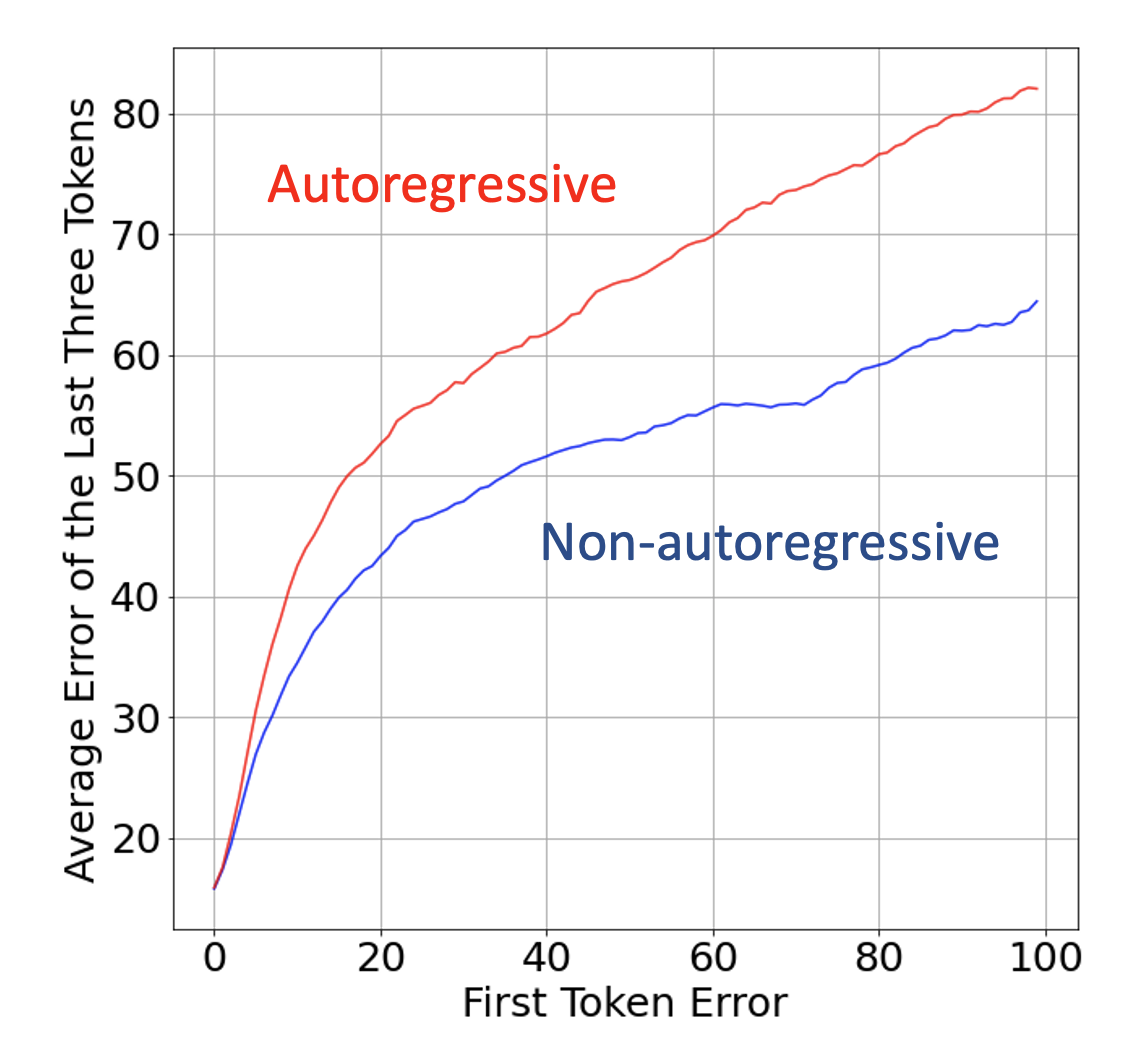}
\end{tabular}
\end{center}
% \vspace{-5mm}
\caption{A Plot to show the effect of the first token error on the remaining sequence tokens. We use RefCOCO dataset here and the sequence is x1, y1, x2, y2 representing the target object bbox. The x-axis ``First Token Error'' is the difference between the predicted x1 coordinate and the ground truth x1 coordinate. The y-axis "Average Error of the Last Three Tokens" is calculated similarly on y1, x2, y2 for samples with higher corresponding first token error value and then we take the average. The errors made on the first token tend to have larger effect on the remaining sequence in AR model, and the gap to NAR model grows as the severity of the first token error increases.
}
% \vspace{-4mm}
%\vspace{2mm}
\label{fig:error_propagation}
\end{figure}

\begin{figure*}[!ht]
%\vspace{-15mm} 
\begin{center}
\begin{tabular} {c}
\includegraphics[width=0.85\textwidth]{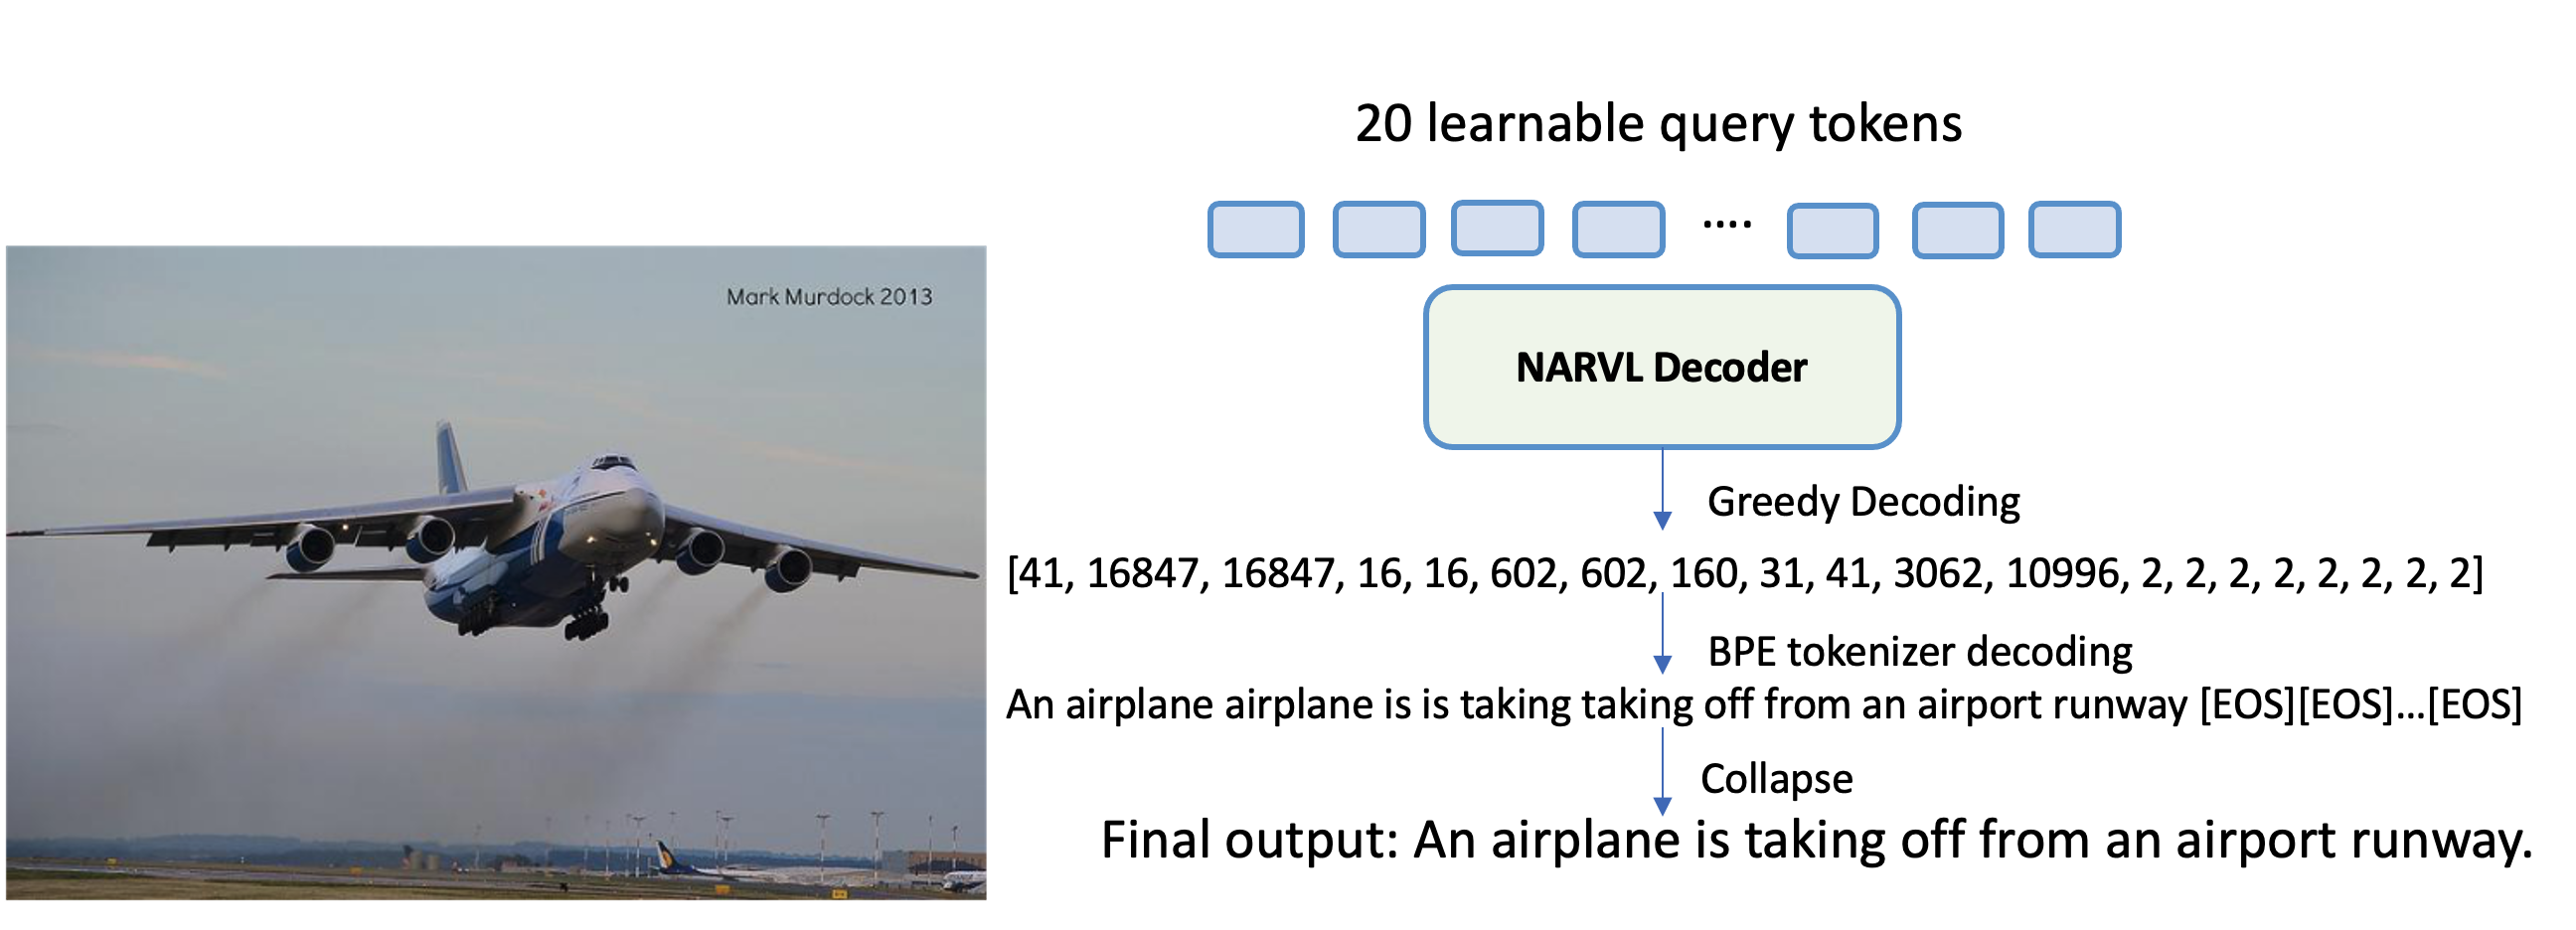} \\
\end{tabular}
\end{center}
% \vspace{-5mm}
\caption{An example to illustrate the whole decoder inference process from learnable query tokens to the final output sequence.
}
% \vspace{-4mm}
%\vspace{2mm}
\label{fig:decodeing_process}
\end{figure*}

\begin{table*}[t]
  \centering
  \scalebox{0.76}{
  \begin{tabular}{ | c | m{10cm} | }
    \hline
    Images & Captions \\ \hline
    \begin{minipage}{.3\textwidth}
      \includegraphics[width=\linewidth]{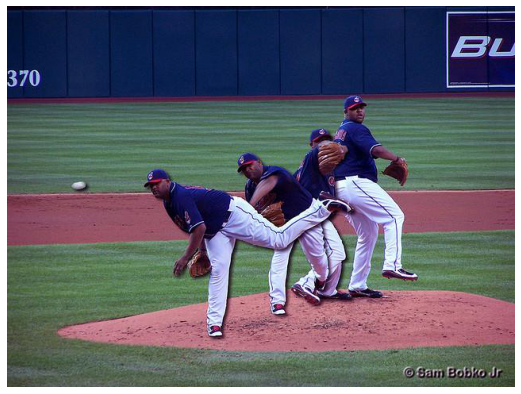}
    \end{minipage}
    &
    %\begin{minipage}[t]{5cm}
      \begin{itemize}
        \item \textbf{CE}: A baseball of players a.
        \item \textbf{Q-CTC}: A baseball of players a on a baseball.
        \item \textbf{Q-CTC+KD}: A group of baseball players on a baseball field. 
        \item \textbf{GT}: Four baseball players pitching balls in the middle of a baseball field.
      \end{itemize}
    %\end{minipage}
    \\ \hline
    
    \begin{minipage}{.3\textwidth}
      \includegraphics[width=\linewidth]{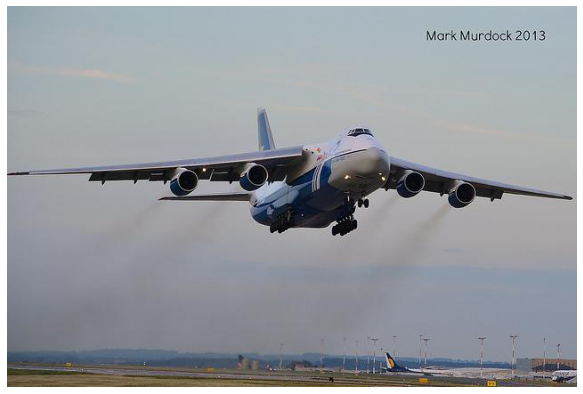}
    \end{minipage}
    &
    %\begin{minipage}[t]{5cm}
      \begin{itemize}
        \item \textbf{CE}: A large jet is the.
        \item \textbf{Q-CTC}: A large airplane jet plane is taking off from the runway.
        \item \textbf{Q-CTC+KD}: An airplane is taking off from an airport runway. 
        \item \textbf{GT}: A large passenger jet taking off from an airport.
      \end{itemize}
    %\end{minipage}
    \\ \hline    

    \begin{minipage}{.3\textwidth}
      \includegraphics[width=\linewidth]{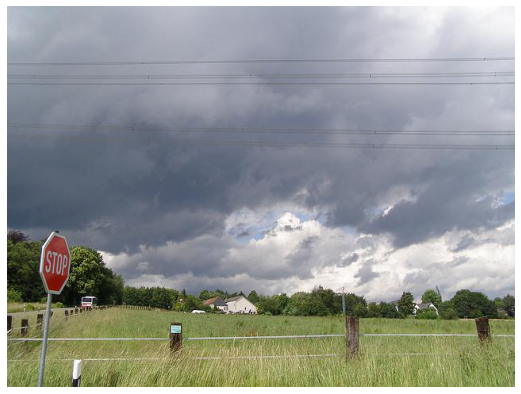}
    \end{minipage}
    &
    %\begin{minipage}[t]{5cm}
      \begin{itemize}
        \item \textbf{CE}: A stop sign a.
        \item \textbf{Q-CTC}: A stop sign a field a cloudy.
        \item \textbf{Q-CTC + KD}: A stop sign in the middle of a field. 
        \item \textbf{GT}: The sky is cloudy over a stop sign.
      \end{itemize}
    %\end{minipage}
    \\ \hline

    \begin{minipage}{.3\textwidth}
      \includegraphics[width=\linewidth]{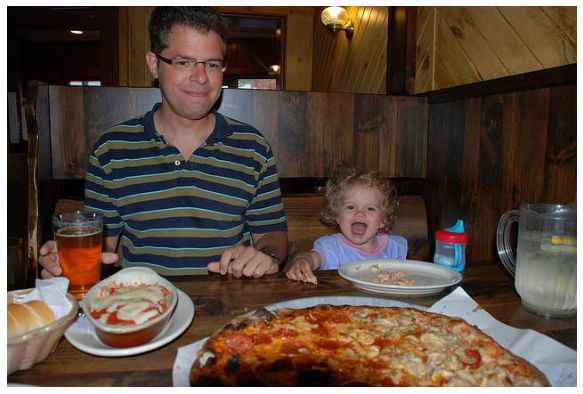}
    \end{minipage}
    &
    %\begin{minipage}[t]{5cm}
      \begin{itemize}
        \item \textbf{CE}: A man and a pizza.
        \item \textbf{Q-CTC}: A man and a table with a pizza.
        \item \textbf{Q-CTC+KD}: A man and a little girl sitting at a table with a pizza. 
        \item \textbf{GT}: A man and a kids at a table with pizza.
      \end{itemize}
    %\end{minipage}
    \\ \hline     
    
    \begin{minipage}{.3\textwidth}
      \includegraphics[width=\linewidth]{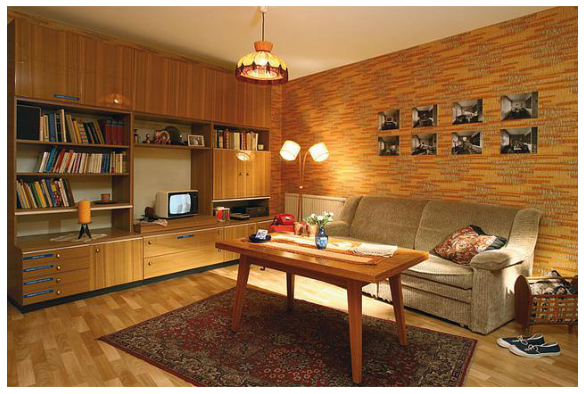}
    \end{minipage}
    &
    %\begin{minipage}[t]{5cm}
      \begin{itemize}
        \item \textbf{CE}: A living room with a and.
        \item \textbf{Q-CTC}: A living room with a and a room.
        \item \textbf{Q-CTC+KD}: A living room with a couch and a table. 
        \item \textbf{GT}: A living room has a couch, a table, and a small television.
      \end{itemize}
    %\end{minipage}
    \\ \hline       
    
  \end{tabular}
  }
  \caption{Qualitative Comparisons of three models on MSCOCO Image Captioning dataset. CE: The first model is trained with cross entropy loss. Q-CTC: The second model is trained with Q-CTC loss. Q-CTC + KD: The third model is trained with Q-CTC loss with knowledge distillation.)}
  \label{table:quali_comp}
\end{table*}

\subsection{Simplified Training Targets with Knowledge Distillation}
\label{sec:kd_effect}
In vision-language tasks, the target sequences often have high freedom, such as multiple captions for a single image, which confuses the model training (see Table \ref{table:distill_cap}). This issue is avoided in auto-regressive model learning, because of the teacher-forcing training schema. However, this issue becomes more serious in NARVL learning. To solve this problem, we use knowledge distillation to reduce the freedom of target sequences. Specifically, we propose to set the sequences predicted by an auto-regressive model as the targets, which are more deterministic compared to the sequences generated by human. Table \ref{table:distill_cap} shows the comparisons of ground truth captions vs the captions generated by an auto-regressive model. 

We also show qualitative result comparisons between the model trained with ground truth and simplified sequences in Table \ref{table:quali_comp}. It can be seen that the model trained with ground truth captions struggles to figure out a mode among all possible valid sequences. In the second example in Table \ref{table:quali_comp}, repetitive description of the same object ``airplane jet plane" might be the consequence of the confusion of training the model with high-freedom target sequences. Such problem is greatly addressed in the model trained with knowledge distillation, and the generated captions are more fluent and cohesive.

\section{NARVL Sequence Decoding Analysis}
In this section, we illustrate sequence generation process in NARVL and study the features of non-autogressive sequences compared to auto-regressive sequences.
\subsection{Sequence generation process}
We illustrate the sequence generation procedure in NARVL. Figure \ref{fig:decodeing_process} contains an example of sequence generation in Image Captioning. The output sequence from NARVL is fixed length and contains repetitive tokens. According the valid path selection rule in Q-CTC loss, we remove the repetitive tokens and output the final sequence.

\subsection{Error Propagation}
\label{sec:error_propagation}
The training of autoregressive model utilizes ground truth tokens as previous tokens, which however are not available at inference time. During inference, the model has to generate the sequence conditioning on previously predicted tokens. The quality of the next predicted tokens depends on the correctness of previous predicted tokens, and the errors might accumulate and propagate via iterations. We study how the previous token errors affect later sequence quality in both AR and NAR models on RefCOCO dataset. We use the value difference between the GT token coordinates and the predicted token coordinates as a measure of the incorrectness (the smaller value difference, the higher correctness), and as shown in Figure \ref{fig:error_propagation}, the first token error in the autoregressive model has higher negative impact on the rest of the sequence.
